# Supplementary material for: Asymptotic Analysis of Equivalences and Core-Structures in Kronecker-Style Graph Models
Source: arXiv:1609.05081 source file (2016-09-16)
Supplement: Supplementary file 1 [file appendix.tex]

\onecolumn
\section*{Appendix}
